# Supplementary material for: Criticality in Reservoir Computer of Coupled Phase Oscillators
Source: arXiv:2108.06395 source file (2021-07-23)
Supplement: Supplementary file 1 [file Supplementary.pdf]

Supplementary Material for  
**Criticality in Reservoir Computer of Coupled Phase Oscillators**

Liang Wang, Huawei Fan, Jinghua Xiao, Yueheng Lan, and Xingang Wang

Corresponding author: X. G. Wang (wangxg@snnu.edu.cn)

**CONTENTS**

|                                                                                                                    |    |
|--------------------------------------------------------------------------------------------------------------------|----|
| I. Impacts of coupling strength on the size distribution of synchronization clusters in generalized Kuramoto model | 2  |
| II. Impacts of parameters $\Delta T$ and $p_c$ on criticality                                                      | 3  |
| III. Prediction performance of the machine under different parameters $\alpha$ , $\beta$ and $\lambda$             | 4  |
| IV. Order parameters of the properly trained machines and the cluster properties                                   | 5  |
| V. Fitting errors of the power-law distributions                                                                   | 6  |
| VI. Impacts of reservoir size on criticality                                                                       | 7  |
| VII. Impacts of simulating time on criticality                                                                     | 9  |
| VIII. Impacts of noise perturbations on criticality                                                                | 9  |
| IX. Results for other Lorenz oscillators                                                                           | 10 |
| X. Results for chaotic Logistic map                                                                                | 11 |

## I. IMPACTS OF COUPLING STRENGTH ON THE SIZE DISTRIBUTION OF SYNCHRONIZATION CLUSTERS IN GENERALIZED KURAMOTO MODEL

In Fig. 1(c) of the main text, the size distribution of the synchronization clusters in the generalized Kuramoto model (i.e., the reservoir without inputs) is presented for several typical coupling strengths, where it is shown that the distribution follows roughly a power-law scaling for  $\alpha = 0.7$  (with the fitted exponent being about  $-1.3$ ). Here we present more results to show that power-law scaling emerges typically in the transition regime  $\alpha \in (0.65, 0.71)$ , but is missing in the desynchronization ( $\alpha < 0.65$ ) and strong-synchronization ( $\alpha > 0.71$ ) regimes. By the same network model and using the same method of cluster identification ( $p_c = 0.95$ ,  $\Delta T = 260$ ), we plot in Fig. S1 the size distribution of the synchronization clusters for different coupling strengths. We see that for coupling strengths in the desynchronization regimes,  $\alpha = (0.2, 0.4, 0.6, 0.64)$ , the distributions are clearly diverged from power-law scalings, as shown in Figs. S1(a-d). When  $\alpha = 0.68$ , the distribution follows approximately a power-law scaling, with the fitted exponent being  $\gamma \approx -1.2$ , as depicted in Fig. S1(e). As  $\alpha$  increases, the fitting is improved, while the scaling exponent is decreased. This is shown in Figs. S1(e-h). Increasing  $\alpha$  to 0.72, the distribution is diverged again from the power-law scaling, as shown in Fig. S1(i). These additional results confirm the generality of criticality in the synchronization transition regime, and show also the dependence of the scaling exponent on the coupling strength in this regime.

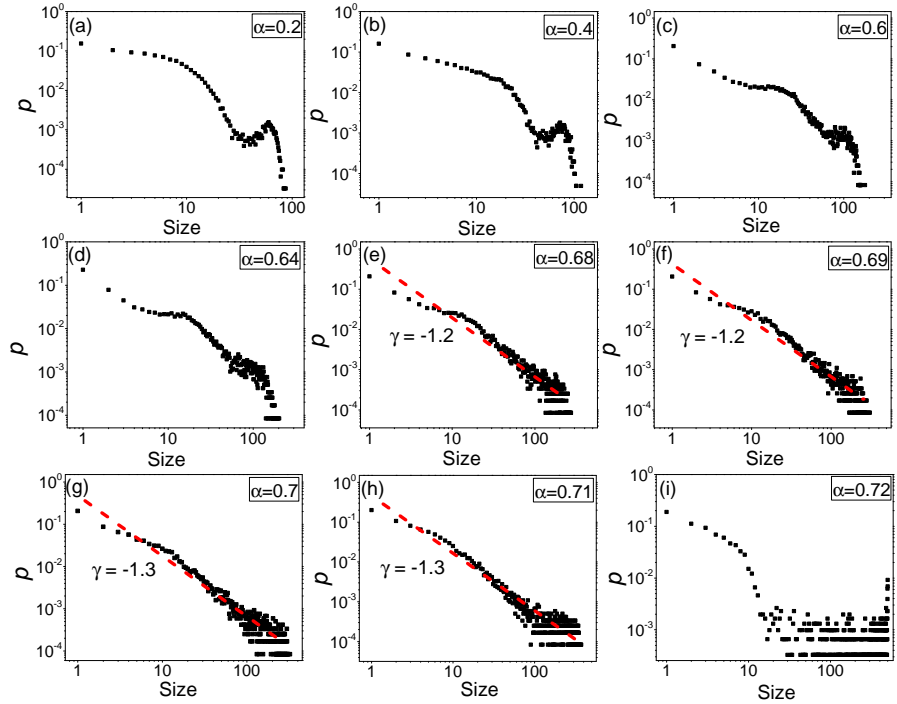

FIG. S1. For the generalized Kuramoto model, the size distribution of the synchronization clusters with different coupling strengths. (a-d) Coupling strengths adopted from the desynchronization regime ( $\alpha < 0.65$ ). The distribution can not be fitted by power-law scaling. (e-h) Coupling strengths adopted from the transition regime ( $\alpha \in (0.65, 0.71)$ ). The distributions can be approximated by power-law scalings, and the scaling exponent is decreased by increasing  $\alpha$ . (i) Coupling strength adopted from the strong-synchronization regime ( $\alpha > 0.71$ ). The distribution can not be fitted by a power-law scaling.

## II. IMPACTS OF PARAMETERS $\Delta T$ AND $p_c$ ON CRITICALITY

In Fig. 2(c) of the main text, a power-law scaling is found in the size distribution of the synchronization clusters for the properly trained machine, in which the parameters used are  $\Delta T = 260$  and  $p_c = 0.95$ . Here we check whether the scaling relationship is affected by the parameters  $\Delta T$  (the time window for calculating the correlation coefficients) and  $p_c$  (the correlation threshold used to define the clusters). Keeping  $p_c = 0.95$  unchanged, we plot in Fig. S2(a) the size distributions for  $\Delta T = 210$  and 310. It is seen that within the interested region  $s \in [1, 80]$ , the distributions are still fitted by a power-law scaling, with the exponent identical to the one for  $\Delta T = 260$ . Fig. S2(a) also shows that the impact of  $\Delta T$  is mainly reflected in the tail of the distribution. Specifically, as  $\Delta T$  increases, the tail is shifted to the left slightly. The shifting is reasonable, as by increasing  $\Delta T$  the probability for generating larger-size clusters will be decreased. Shown in Fig. S2(b) is the size distributions for different values of  $p_c$ , while  $\Delta T$  is fixed as 260. Still, we observe that the distributions follow the power-law scaling,  $p_s \propto s^{-1.7}$ .

In Fig. 2(f) of the main text, it is shown that for the case of poorly trained machine, the size distribution of the synchronization clusters can not be fitted by a power-law scaling when the parameters are chosen as  $\Delta T = 260$  and  $p_c = 0.95$ . Here we provide more evidences to show the absence of criticality in this poorly trained machine. That is, despite the variations of  $\Delta T$  and  $p_c$ , the power-law scaling is always absent in the distribution if the machine is not properly trained. The results are plotted in Fig. S3.

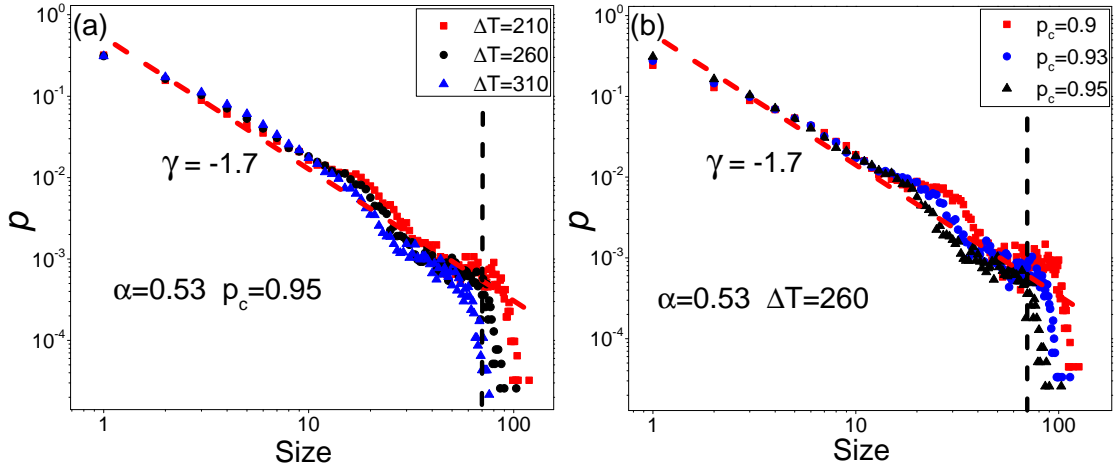

FIG. S2. *The criticality is independent on the parameters  $\Delta T$  and  $p_c$ .* The RC and target system are identical to the ones used in Fig. 2(c) in the main text, in which the size distribution of the synchronization clusters follows a power-law scaling with the parameters  $\Delta T = 260$  and  $p_c = 0.95$ . (a) Fixing  $p_c = 0.95$ , the size distributions for different values of  $\Delta T$ . (b) Fixing  $\Delta T = 260$ , the size distributions for different values of  $p_c$ .

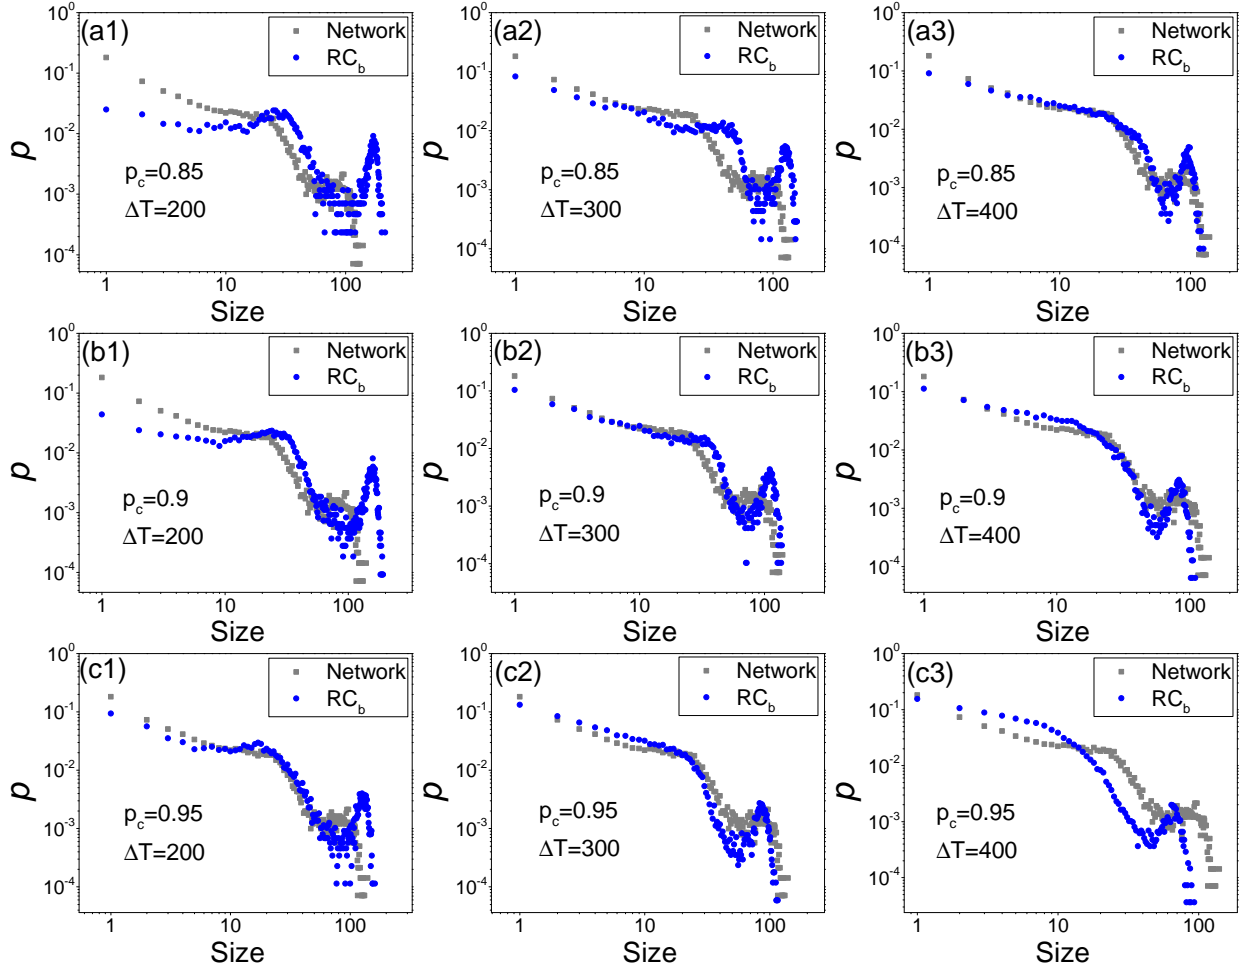

FIG. S3. *Criticality is absent in the poorly trained machine.* The RC and target system are identical to the ones used in Fig. 2(f), in which the size distribution of the synchronization clusters can not be fitted by a power-law scaling for the parameters  $\Delta T = 260$  and  $p_c = 0.95$ . Shown are the size distributions under different values of  $\Delta T$  and  $p_c$  for the poorly trained machine. It is seen that, despite the variations of  $\Delta T$  and  $p_c$ , the distribution is always clearly different from the power-law distribution. Grey discs: the size distribution of the synchronization clusters for the original reservoir network (without inputs) with the coupling strength  $\alpha = 0.53$ .

### III. PREDICTION PERFORMANCE OF THE MACHINE UNDER DIFFERENT PARAMETERS $\alpha$ , $\beta$ AND $\lambda$

Our main finding in the present work is the universality of criticality in properly trained machines, i.e., the results plotted in Fig. 3 in the main text. In our studies, a machine is regarded as properly trained if it is able to predict the state evolution of the target system for several Lyapunov times. Here we show the prediction performance of the machines reported in Fig. 3 in the main text. The results are plotted in Fig. S4 in this reply. We see that, all the machines are able to predict the state evolution of the chaotic Lorenz oscillator for at least 6 Lyapunov times, i.e., all machines listed in Fig. 3 in the main text are properly trained.

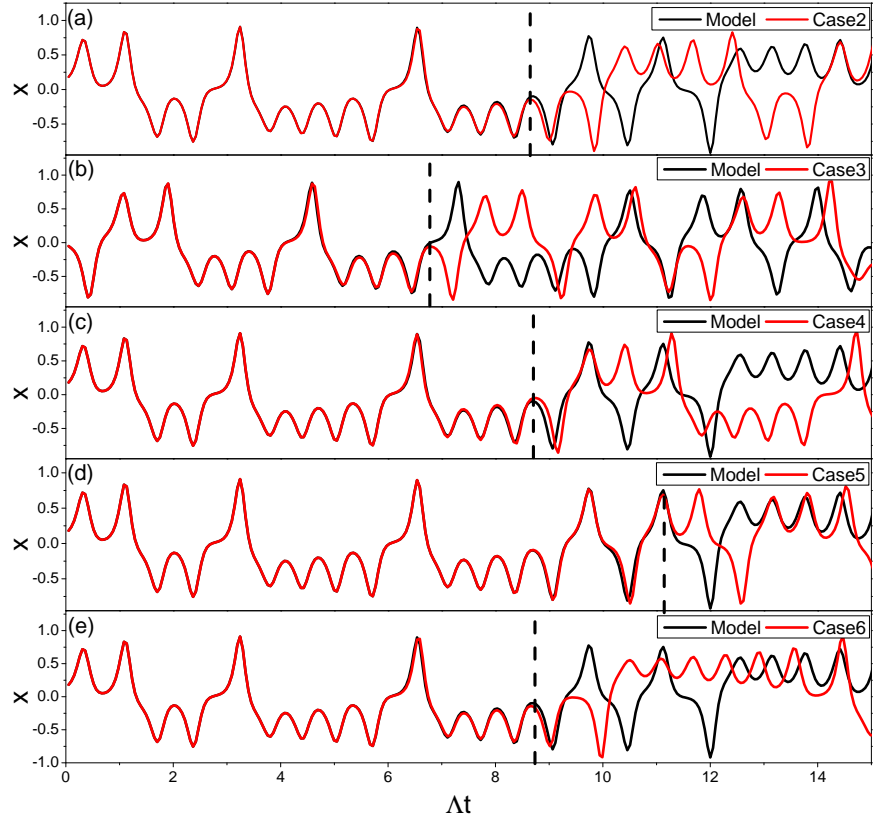

FIG. S4. *Prediction performance of the properly trained machines shown in Fig. 3 in the main text.* Shown is the time evolution of the variable  $x$  predicted by the machine in different cases. The parameters of the RCs are identical to the ones used in Fig. 3 in the main text. Case 2:  $\alpha = 0.53$ ,  $(\beta, \lambda) = (0.254, 3 \times 10^{-7})$ . Case 3:  $\alpha = 0.53$ ,  $(\beta, \lambda) = (0.371, 1 \times 10^{-7})$ . Case 4:  $\alpha = 0.25$ ,  $(\beta, \lambda) = (0.215, 1 \times 10^{-7})$ . Case 5:  $\alpha = 0.7$ ,  $(\beta, \lambda) = (0.448, 1 \times 10^{-7})$ . Case 6:  $\alpha = 0.8$ ,  $(\beta, \lambda) = (0.616, 1 \times 10^{-7})$ . In all the cases, the machine is able to predict the state evolution accurately for at least 6 Lyapunov times.

#### IV. ORDER PARAMETERS OF THE PROPERLY TRAINED MACHINES AND THE CLUSTER PROPERTIES

When the machine is properly trained, the size distribution of the synchronization clusters will be “shaped” to the same power-law scaling, as shown in Fig. 3 in the main text. In our studies, it is also found that when the machine is properly trained, the order parameter of the reservoir network is decreased, as compared to the order parameter of the original network without inputs. The order parameters of the properly trained machines are given in Tab. S1 in this reply, in which  $r_{original}$  and  $r_{trained}$  denote, respectively, the order parameters of the original network and the reservoir of properly trained machine. The cases listed in the table are identical to the ones shown in Fig. 3 in the main text. We see that except case 4 in which the order parameter only decreased slightly [with the parameters  $(\alpha, \beta, \lambda) = (0.25, 0.215, 1 \times 10^{-7})$ ], in all other cases the order parameter of the trained machine is clearly smaller than that of the original network.

The decreased order parameter in the reservoir of properly trained machine is attributed to the breaking of the giant synchronization clusters. To demonstrate this, we monitor the time evolutions of the number of synchronization clusters and the size of the largest synchronization

TABLE S1. Order parameter of the reservoir network in properly trained machine under different RC parameters.  $r_{original}$  denotes the order parameter of the original reservoir without inputs, i.e., the generalized Kuramoto model.  $r_{trained}$  denotes the order parameter of reservoir for the properly trained machine.  $\langle s \rangle_{original}$  and  $\langle s \rangle_{trained}$  represent, respectively, the average size of the clusters in the original network and the properly trained machine.  $\hat{D}$  is the normalized distance used to evaluate the precision of the fittings. The cases are identical to the ones plotted in Fig. 3 in the main text.

| Cases  | RC parameters                                                | $r_{original}$ | $r_{trained}$ | $\langle s \rangle_{original}$ | $\langle s \rangle_{trained}$ | $\hat{D}$ |
|--------|--------------------------------------------------------------|----------------|---------------|--------------------------------|-------------------------------|-----------|
| Case 1 | $(\alpha, \beta, \lambda) = (0.53, 0.477, 2 \times 10^{-5})$ | 0.071          | 0.0397        | 17.7                           | 6.42                          | 0.28      |
| Case 2 | $(\alpha, \beta, \lambda) = (0.53, 0.254, 3 \times 10^{-7})$ | 0.071          | 0.0396        | 17.7                           | 7                             | 0.36      |
| Case 3 | $(\alpha, \beta, \lambda) = (0.53, 0.371, 1 \times 10^{-7})$ | 0.071          | 0.0403        | 17.7                           | 7.27                          | 0.32      |
| Case 4 | $(\alpha, \beta, \lambda) = (0.25, 0.215, 1 \times 10^{-7})$ | 0.046          | 0.04          | 8.82                           | 7.8                           | 0.4       |
| Case 5 | $(\alpha, \beta, \lambda) = (0.7, 0.448, 1 \times 10^{-7})$  | 0.322          | 0.0398        | 20.95                          | 7.12                          | 0.31      |
| Case 6 | $(\alpha, \beta, \lambda) = (0.8, 0.616, 1 \times 10^{-7})$  | 0.952          | 0.0384        | 152.74                         | 6.18                          | 0.29      |

cluster in the reservoir for three cases: the original network (without inputs), the properly trained machine ( $RC_g$ ), and the poorly trained machine ( $RC_b$ ). The results for  $\alpha = 0.53$  are shown in Fig S5(a) in this reply. (The cluster-size distribution of the three cases are shown in Fig. 2 in the main text.) We see that for the original network and  $RC_b$ , the oscillators are synchronized into a small number of clusters ( $\sim 20$ ) [Fig. S5(a1)] and the largest cluster contains more than 100 oscillators [Fig. S5(a2)]. However, when the machine is properly trained ( $RC_g$ ), the oscillators are synchronized to a large number of clusters ( $\sim 80$ ) [Fig. S5(a1)] and the largest cluster contains only about 60 oscillators [Fig. S5(a2)]. The similar results are also observed for  $\alpha = 0.8$ , as shown in Fig. S5(b). In particular, for the case of  $\alpha = 0.8$ , oscillators in the original network are frequently synchronized into a single cluster (indicating the strong synchronization of the network), while in the properly trained machine, the network contains about 80 small-size clusters, with the largest cluster contains only about 60 oscillators.

As a consequence of cluster breaking, the average size of the synchronization clusters in the reservoir network,  $\langle s \rangle = \sum_s s p_s$ , is decreased. The results are given in Tab. S1, in which  $\langle s \rangle_{original}$  and  $\langle s \rangle_{trained}$  represent, respectively, the average size of the clusters in the original network (reservoir without inputs) and the properly trained machine.

## V. FITTING ERRORS OF THE POWER-LAW DISTRIBUTIONS

The power-law scalings shown in Fig. 3 in the main text are obtained by the least-square fitting over the range  $s \in [1, 70]$ . Following the studies in neuroscience, we use the normalized distance to evaluate the error of the fittings. The normalized distance is defined as  $\hat{D} = \sum_s s |p_s - p_s^{fit}| / \sum_s s p_s$ , with  $p_s^{fit}$  the fitted probability for finding a cluster of size  $s$ . Briefly,  $\hat{D}$  measures the difference between the averaged sizes of the synchronization clusters,  $\langle s \rangle = \sum_s s p_s$ , between the actual and fitted results. The smaller the value of  $\hat{D}$ , the better the fitting. This quantity is essentially the same as the widely used  $\kappa$ -index in assessing criticality in experimental studies (see, for example, Refs. [33-41] in the main text), but requiring no pre-definition of the scaling exponent. The fitting

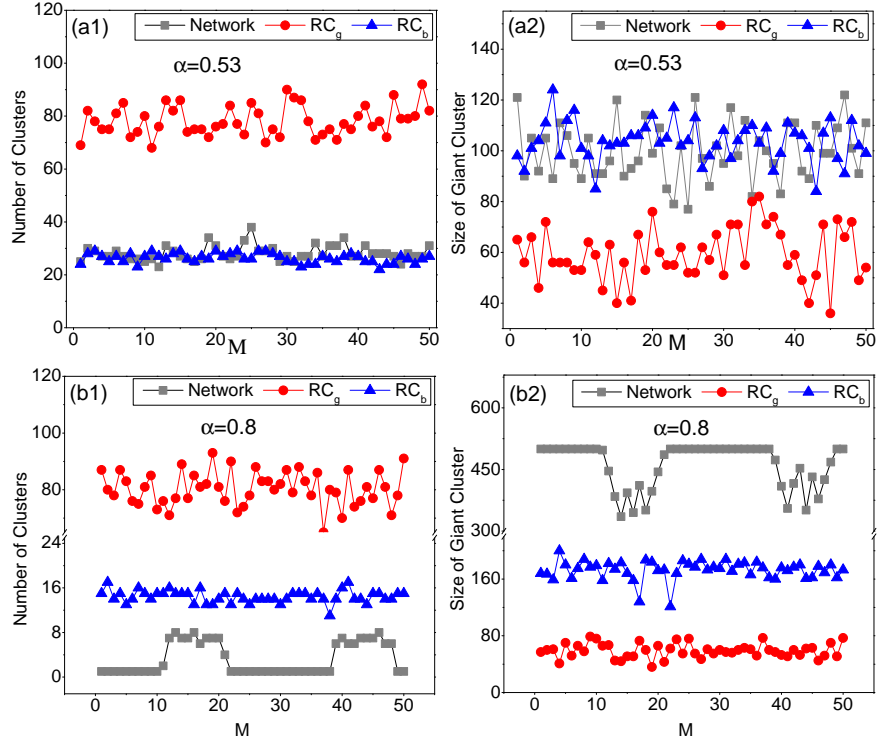

FIG. S5. Time evolutions of the number of synchronization clusters and the size of the largest synchronization cluster in the reservoir network. (a) The results for  $\alpha = 0.53$ . The order parameters of the original network, the poorly trained machine ( $RC_b$ ) and the properly trained machine ( $RC_g$ ) are, respectively, 0.071, 0.07 and 0.0397. (b) The results for  $\alpha = 0.8$ . The order parameters of the original network, the poorly trained machine ( $RC_b$ ) and the properly trained machine ( $RC_g$ ) are, respectively, 0.952, 0.841 and 0.0384. Grey squares: results for the original network. Red discs: results for the properly trained machine. Blue triangles: results for the poorly trained machine.  $M$  denotes the time index of the synchronization patterns.

errors of the scalings shown in Fig. 3 in the main text are given in Tab. S1 (the last column).

## VI. IMPACTS OF RESERVOIR SIZE ON CRITICALITY

The results reported in the main text are obtained for reservoir network of size  $N = 500$ . Here we show that the results are independent on the network size. To demonstrate, we keep the other parameters of the reservoir network unchanged, while increasing the network size to  $N = 800$ . Still, the network dynamics is described by the generalized Kuramoto model, as did in Figs. 1-3 in the main text. The variation of the synchronization order parameter  $r$  with respect to the coupling strength  $\alpha$  is plotted in Fig. S6(a). We see that the order parameter is quickly increased with  $\alpha$  in the transition regime  $\alpha \in (0.7, 0.72)$ . In constructing the RC, we set  $\alpha = 0.5$  for the reservoir, by which the order parameter is about 0.05, i.e., the original network (without input) is desynchronized. The target system is still chosen as the chaotic Lorenz oscillator ( $p = 35$ ). The case of properly trained machine is shown in Fig. S6(b). We see that the machine is able to predict the system evolution for about 11 Lyapunov times [see Fig. S6(b1)]. The size distribution of the synchronization clusters for the properly trained machine is plotted in Fig. S6(b2), in which

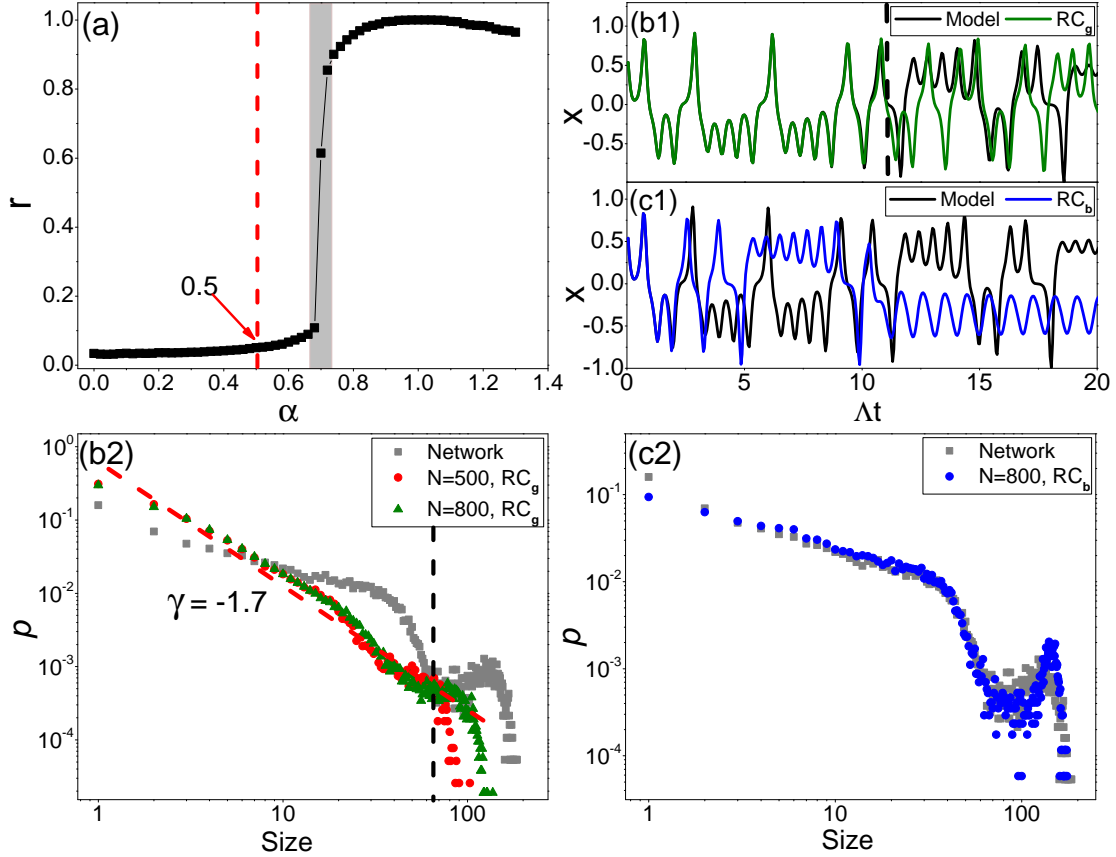

FIG. S6. *Results for reservoir network of size  $N = 800$ .* (a) The variation of the synchronization order parameter  $r$  with respect to the coupling strength  $\alpha$ . The transition regime is approximately  $\alpha \in (0.7, 0.72)$  (the grey zone).  $r \approx 0.05$  at  $\alpha = 0.5$ . (b) The prediction performance and criticality feature of a properly trained machine. The parameters are  $(N, \alpha, \beta, \lambda) = (800, 0.5, 0.36, 4 \times 10^{-8})$ . (b1) The time evolution of variable  $x$  predicted by the machine. (b2) The size distribution of the synchronization clusters for the properly trained machine. The results for  $N = 500$  are shown in red. (c) The results for a poorly trained machine with the RC parameters  $(N, \alpha, \beta, \lambda) = (800, 0.5, 0.375, 1 \times 10^{-3})$ . In (b2) and (c2), the size distribution of the clusters for the original network with coupling strength  $\alpha = 0.5$  (reservoir without input) is shown as grey squares.

the parameters used for identifying the synchronization clusters are still chosen as  $\Delta T = 260$  and  $p_c = 0.95$ . We see that within the range  $s \in [1, 100]$ , the distribution follows a power-law scaling  $p_s \propto s^\gamma$ , with the fitted exponent being  $\gamma \approx -1.7$ . As a comparison, we plot in Fig. S6(b2) also the results for  $N = 500$  (copied from Fig. 2(c) in the main text). We see that the two distributions are well overlapped in the region  $s \in [1, 70]$ . The main difference is reflected in the tail, which is right-shifted for  $N = 800$ . The case of poorly trained machine is presented in Figs. S6(c1) and (c2). We see that the machine is able to predict the evolution for only about 2 Lyapunov time, and criticality is absent, i.e., the size distribution of the synchronization clusters can not be fitted by a power-law scaling.

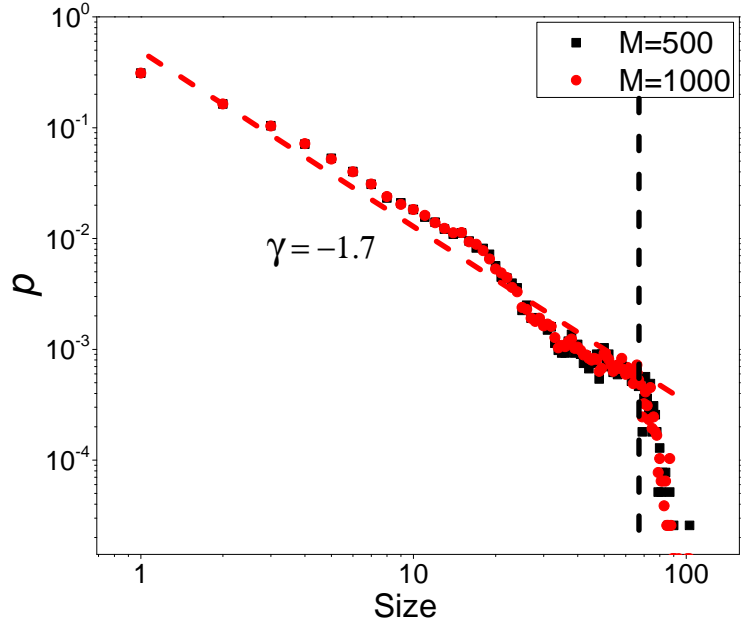

FIG. S7. *Impacts of simulating time on criticality.* Shown is the size distribution of the synchronization clusters for the properly trained machine (the one used in generating Fig. 2(c) in the main text) analyzed over  $M = 1000$  temporal synchronization patterns. The results obtained from  $M = 500$  patterns are shown in black. We see that the increase of the simulating time does not affect the scaling property.

## VII. IMPACTS OF SIMULATING TIME ON CRITICALITY

In obtaining the size distribution of the synchronization clusters, a total number of  $M = 500$  segments (patterns) have been analyzed in the main text. To test whether the scaling property of the distribution is affected by the number of patterns used in the analysis, we extend the simulating time to be containing  $M = 1000$  segments, and analyze again the size distribution of the synchronization clusters. The results are shown in Fig. S7 in this reply. We see that the increase of the simulating time does not affect the scaling property of the distribution.

## VIII. IMPACTS OF NOISE PERTURBATIONS ON CRITICALITY

To check the impacts of noise perturbations on criticality, we modify the dynamics of the phase oscillators to

$$\dot{\theta}_i(t) = (1 - \alpha)\omega_i + \frac{\alpha}{N} \sum_{j=1}^N a_{ij} \sin[\theta_j(t) - \theta_i(t)] + \beta \tanh \left[ b_i + \sum_{j=1}^{D_{in}} h_{ij} u_j(t) \right] + D\eta(t). \quad (\text{S8.1})$$

Here  $\eta(t)$  is the Gaussian white noise, with  $\langle \eta(t) \rangle = 0$  and  $\langle \eta(t)\eta(t') \rangle = \delta(t - t')$ .  $D$  denotes the noise amplitude. The trained RC is identical to the one used in Figs. 2 (a-c) in the main text, i.e., the case of properly trained machine capable of predicting the evolution of chaotic Lorenz oscillator for about 10 Lyapunov times [see Fig. 2(a) in the main text] and oscillators in the reservoir network show the feature of criticality [see Fig. 2(c) in the main text]. Setting  $D = 1 \times 10^{-2}$ , we plot in Figs. S8(a) the state evolution predicted by the machine. We see that the prediction

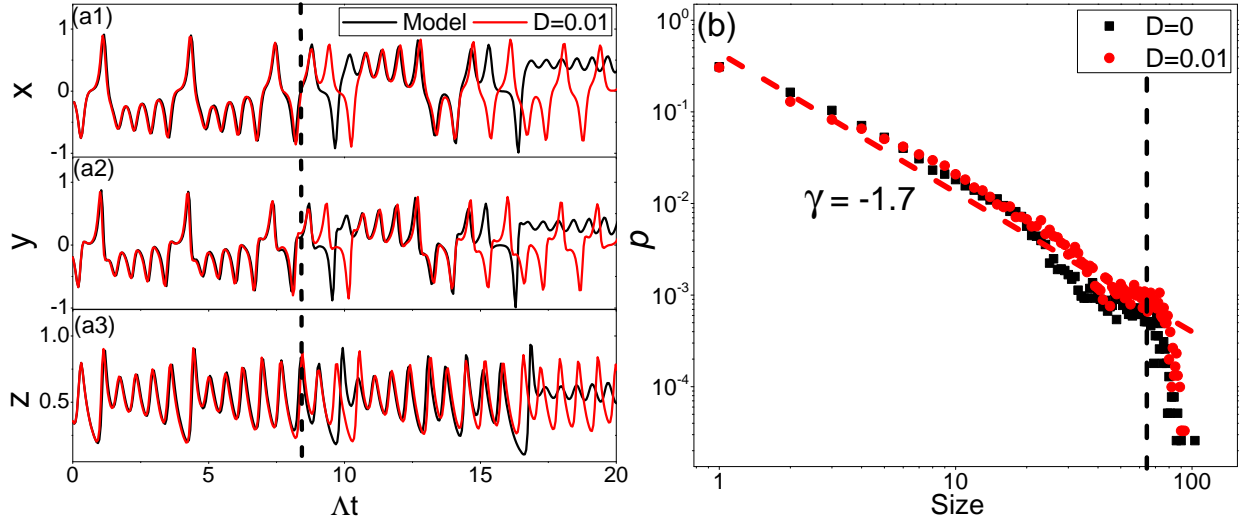

FIG. S8. *Impacts of noise perturbations on criticality.* With noise amplitude  $D = 0.01$ , the state evolution predicted by the machine (a) and the size distribution of the synchronization clusters (b). Comparing to the results of noise-free reservoir ( $D = 0$ ), the prediction horizon is slightly decreased, while the scaling property of the distribution is almost unchanged.

horizon is about 8 Lyapunov times, which is slightly below the one without noise perturbations (about 10 Lyapunov times). The size distribution of the synchronization clusters is plotted in Fig. S8(b). We see that the size distribution follows still the power-law scaling  $p_s \propto s^\gamma$ , with  $\gamma \approx -1.7$ . We note that criticality is observable for only weak noise perturbations. When  $D$  is large, e.g.,  $D = 0.2$ , the state predicted by the machine will be diverging. In such a case, criticality is absent in the reservoir network.

## IX. RESULTS FOR OTHER LORENZ OSCILLATORS

We have shown that the size distribution of the synchronization clusters is independent on the RC parameters, as depicted in Fig. 3 in the main text. Here we show that the scaling property is also independent on the bifurcation parameters of the target system. In particular, given the target system is governed by the same type of dynamics, criticality of the same scaling exponent will be always emerged in the reservoir of properly trained machines. Setting  $\rho = 313$ , the motion of the Lorenz oscillator is periodic, as shown in Fig. S9(a1). The state evolution of the periodic oscillator predicted by the machine is plotted in Fig. S9(a2). The size distribution of the synchronization clusters in the reservoir network is plotted in Fig. S9(a3). We see that the machine is properly trained and the distribution follows the power-law scaling  $p_s \propto s^{-1.7}$  in the region  $s \in [1, 70]$ , which is identical to the one shown in Fig. 3 in the main text (in which the bifurcation parameter of the target system is  $\rho = 35$ ). To show an additional example, we set  $\rho = 60$  for the Lorenz oscillator, by which the oscillator is chaotic and the largest Lyapunov exponent of the oscillator is about 1.44 [see Fig. S9(b1) for the attractor]. Shown in Fig. S9(b2) is the state evolution of the oscillator predicted by the machine. We see that the prediction horizon is about 7 Lyapunov times. The size distribution of the synchronization cluster in the reservoir is plotted in Fig. S9(b3). We see that the distribution also follows a power-law scaling  $p_s \propto s^\gamma$ , with  $\gamma \approx -1.7$ .

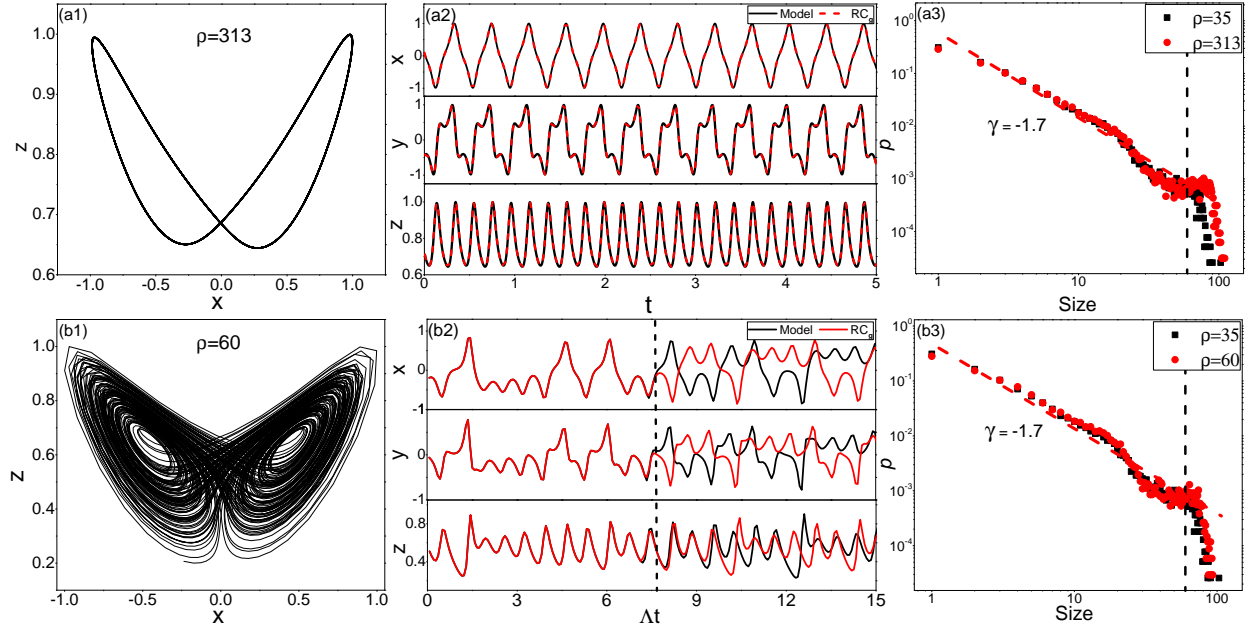

FIG. S9. *Results for other Lorenz oscillators.* (a) The results for periodic Lorenz oscillator generated by parameter  $\rho = 313$ . (a1) The periodic oscillator. (a2) The state evolution of the periodic oscillator predicted by the machine. The RC parameters are  $(N, \alpha, \beta, \lambda) = (500, 0.53, 0.35, 9 \times 10^{-5})$ . (a3) The size distribution of synchronization clusters in the reservoir network, which follows roughly the power-law scaling  $p_s \propto s^\gamma$ , with  $\gamma \approx -1.7$ . (b) The results for chaotic Lorenz oscillator generated by parameter  $\rho = 60$ . (b1) The chaotic oscillator. (b2) The state evolution predicted by the machine. The RC parameters are  $(N, \alpha, \beta, \lambda) = (500, 0.53, 0.36, 1 \times 10^{-7})$ . (b3) The size distribution of synchronization clusters, which follows roughly the power-law scaling  $p_s \propto s^{-1.7}$ . In (a3) and (b3), the black samples are the results for the chaotic Lorenz oscillator ( $\rho = 35$ ) studied in the main text. We see that the scaling property is independent on the bifurcation parameter of the target system.

## X. RESULTS FOR CHAOTIC LOGISTIC MAP

In the main text, the criticality is demonstrated for two types of time-continuous target systems, namely the chaotic Lorenz and Rössler oscillators. Here we demonstrate the criticality in learning time-discrete systems. As an illustration, we choose the chaotic Logistic map:  $x_{n+1} = 4x_n(1 - x_n)$ . The Lyapunov exponent of the map is about 0.69. The other parameters of the RC are identical to the ones used the main text, except the parameters  $\beta$  and  $\lambda$ . Setting  $(\beta, \lambda) = (0.35, 2.7 \times 10^{-4})$ , the machine is properly trained, as depicted in Fig. S10(a) in this reply (the prediction horizon is about 10 iterations). The return map constructed from the predictions is plotted in Fig. S10(b). We see the points are well settled onto the curve described by the function  $x_{n+1} = 4x_n(1 - x_n)$ . The size distribution of the synchronization clusters is plotted in Fig. S10(c). We see that the distribution can be approximated by a power-law scaling  $p_s \propto s^\gamma$ , with  $\gamma \approx -1.6$ .

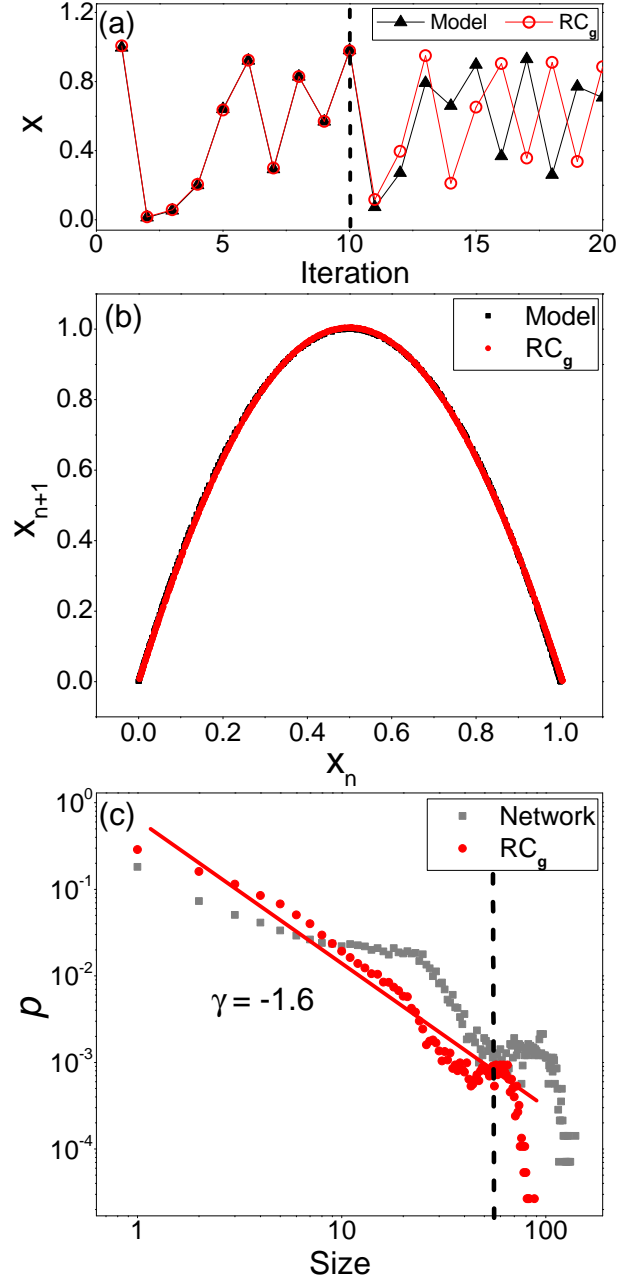

FIG. S10. *Results for chaotic Logistic map.* The RC parameters are  $(N, \alpha, \beta, \lambda) = (500, 0.53, 0.35, 2.7 \times 10^{-4})$ . (a) The state evolution predicted by the machine. (b) The return map constructed from the RC outputs. Black squares denote the mapping function  $x_{n+1} = 4x_n(1 - x_n)$ . (c) The size distribution of the synchronization clusters in the reservoir network. The distribution follows roughly the power-law scaling  $p_s \propto s^{-1.6}$ . Grey squares: the distribution of the original reservoir network (without inputs) with the coupling strength  $\alpha = 0.53$ .
